# Supplementary material for: A detailed introduction to density-based topology optimisation of fluid flow problems with implementation in MATLAB
Source: arXiv:2207.13695 source file (2022-07-19)
Supplement: Supplementary file 1 [file supplementary_codeDescription.pdf]

# Description of MATLAB code for density-based topology optimisation of fluid flow problems

Joe Alexandersen
Department of Mechanical and Electrical Engineering
University of Southern Denmark
Campusvej 55, DK-5230 Odense M, Denmark
Tel.: +45 65507465, e-mail: joalsdu.dk

June 1, 2022

**Abstract**

This is a detailed description of the code provided with the publication "A detailed introduction to density-based topology optimisation of fluid flow problems with implementation in MATLAB", doi: XXX.

# 1 Detailed description of `topFlow.m`

## 1.1 Definition of input parameters (lines 6-29)

The first part of the code is where various input parameters are set to define the physical problem and the optimisation settings.

Two different problems are already implemented and the `probtype` variable determines which one is to be optimised:

```
7  % PROBLEM TO SOLVE (1 = DOUBLE PIPE; 2 = PIPE BEND)
8  probtype = 1;
```

Next the dimensions of the domain and the discretisation are given:

```
9  % DOMAIN SIZE
10 Lx = 1.0; Ly = 1.0;
11 % DOMAIN DISCRETISATION
12 nely = 30; nelx = nely*Lx/Ly;
```

where `Lx` and `Ly` are the dimensions in the $x$- and $y$-directions, respectively. The number of elements in the x-direction, `nelx`, is automatically determined from the supplied number of elements in the y-direction, `nely`, to ensure square elements. The implementation can handle rectangular elements, so `nelx` can be decoupled from `nely` if necessary.

The allowable volume fraction $V_f$ is stored in the `volfrac` variable and the initial design field value is set to be the same to fulfill the volume constraint from the start:

```
% ALLOWABLE FLUID VOLUME FRACTION
volfrac = 1/3; xinit = volfrac;
```

The inlet velocity $U_{in}$ is stored in the variable `Uin` and the fluid density, $\rho$ and dynamic viscosity, $\mu$, are stored in the variables `rho` and `mu`, respectively:

```
% PHYSICAL PARAMETERS
Uin = 1e0; rho = 1e0; mu = 1e0;
```

The maximum and minimum Brinkman penalty factors are per default defined with respect to an out-of-plane thickness according to Equation 9 of the manuscript and the heuristic continuation scheme is automatically computed and stored in `qavec`:

```
% BRINKMAN PENALISATION
alphamax = 2.5*mu/(0.01^2); alphamin = 2.5*mu/(100^2);
% CONTINUATION STRATEGY
ainit = 2.5*mu/(0.1^2);
qinit = (-xinit*(alphamax-alphamin) - ainit + ...
    alphamax)/(xinit*(ainit-alphamin));
qavec = qinit./[1 2 10 20]; qanum = length(qavec); conit = 50;
```

where `ainit` is the initial Brinkman penalty, `qinit` is the initial interpolation factor computed using Equation ??, `qanum` is the number of continuation steps, and `conit` is the maximum number of iterations per continuation step.

Various optimisation parameters are then defined:

```
% OPTIMISATION PARAMETERS
maxiter = qanum*conit; mvlim = 0.2; plotdes = 0;
chlim = 1e-3; chnum = 5;
```

where `maxiter` is the maximum number of total design iterations, `mvlim` is the movelimit $m$ for the OC update, `chlim` is the stopping criteria, `chnum` is the number of subsequent iterations the convergence criteria must be met, and `plotdes` is a Boolean determining whether to plot the design during the optimisation process ($0 = $ no, $1 = $ yes).

The parameters for the Newton solver are defined:

```
26 % NEWTON SOLVER PARAMETERS
27 nltol = 1e-6; nlmax = 25; plotres = 0;
```

where `nltol` is the required residual tolerance for convergence, `nlmax` is the maximum number of non-linear iterations, and `plotres` is a Boolean determining whether to plot the convergence of the residual norm over the optimisation process (0 = no, 1 = yes).

Finally, the option to export the contour of the final design as a DXF (Data Exchange Format) file can be activated:

```
28 % EXPORT FILE
29 filename='output'; exportdxf = 0;
```

where `filename` is a specified filename and `exportdxf` is a Boolean determining whether to export the design (0 = no, 1 = yes).

## 1.2 Pre-processing (lines 30-71)

### 1.2.1 Preparation of finite element analysis (lines 30-44)

Firstly, mesh variables are calculated from the specified problem dimensions and discretisation:

```
30 %% PREPARE FINITE ELEMENT ANALYSIS
31 dx = Lx/nelx; dy = Ly/nely;
32 nodx = nelx+1; nody = nely+1; nodtot = nodx*nody;
33 neltot = nelx*nely; doftot = 3*nodtot;
```

where `dx` is the element width, `dy` is the element height, `nodx` is the number of nodes in the $x$-direction, `nody` is the number of nodes in the $y$-direction, and `nodtot`, `neltot` and `doftot` are the total number of nodes, elements and DOFs, respectively.

The nodal connectivity and various DOF mappings are then automatically set up based on the approach outlined by **?**:

```
34 % NODAL CONNECTIVITY
35 nodenrs = reshape(1:nodtot,nody,nodx);
36 edofVecU = reshape(2*nodenrs(1:end-1,1:end-1)+1,neltot,1);
37 edofMatU = repmat(edofVecU,1,8)+repmat([0 1 2*nely+[2 3 0 1] ...
      -2 -1],neltot,1);
38 edofVecP = reshape(nodenrs(1:end-1,1:end-1),neltot,1);
39 edofMatP = repmat(edofVecP,1,4)+repmat([1 nely+[2 1] ...
      0],neltot,1);
40 edofMat = [edofMatU 2*nodtot+edofMatP];
```

where `edofMatU` is a `neltot` $\times$ 8 matrix containing the velocity DOF numbering for each element, `edofMatP` is a `neltot` $\times$ 4 matrix containing the

pressure DOF numbering for each element, and `edofMat` is a `neltot` $\times$ 12 matrix containing all DOFs for each element.

Finally, the triplet information to build the sparse matrices and vectors needs to be computed:

```
41 iJ = reshape(kron(edofMat,ones(12,1))',144*neltot,1);
42 jJ = reshape(kron(edofMat,ones(1,12))',144*neltot,1);
43 iR = reshape(edofMat',12*neltot,1); jR = ones(12*neltot,1);
44 jE = repmat(1:neltot,12,1);
```

where `iJ` and `jJ` are the first and second subscript positions for the Jacobian matrix, respectively, `iR` and `jR` are the first and second (all ones) subscript positions for the residual vector, respectively, and `jE` is the second subscript position for the $\frac{\partial \mathbf{r}}{\partial \gamma}$ matrix.

### 1.2.2 Definition of boundary conditions (lines 45-51)

The boundary conditions for fluid flow problems are typically more complex than for static elasticity, so the definition of the fixed DOFs and their values are defined in a separate script to keep the main code clean and readable:

```
46 % DEFINE THE PROBLEMS IN SEPARATE MATLAB FILE
47 run('problems.m');
```

Hereafter, the nullspace matrices are defined to impose the boundary conditions:

```
48 % NULLSPACE MATRICES FOR IMPOSING BOUNDARY CONDITIONS
49 EN=speye(doftot); ND=EN; ND(fixedDofs,fixedDofs)=0.0; EN=EN-ND;
```

Finally, the free DOFs are computed:

```
50 % VECTORS FOR FREE DOFS
51 alldofs = 1:doftot; freedofs = setdiff(alldofs,fixedDofs);
```

based on the fixed DOFs defined in the `fixeddofs` vector in `problems.m`.

The problem definition script `problems.m` contains two problems, where the setup of the double pipe problem will be covered in Section 2.

### 1.2.3 Initialisation (lines 52-66)

Before starting the optimisation loop, several variables and vectors need to be initialised. Firstly, the state and adjoint solution vectors are initialised:

```
53 % SOLUTION VECTOR
54 S = zeros(doftot,1); dS = S; L = S;
55 S(fixedDofs) = DIR(fixedDofs);
```

where `S` is the state solution vector, `dS` is the Newton step vector, and `L` is the adjoint solution vector. The fixed DOFs of the system are set to be identical to the imposed values, which ensures the boundary conditions are fulfilled from the start.

The design field (`xPhys`) is initialised to start with the initial value `xinit` defined previously:

```
56 % DESIGN FIELD
57 xPhys = xinit*ones(nely,nelx);
```

Various counters and variables that need initial values are initiated in lines 58-63. In order for efficiently building the element vectors using the vectorised functions generated by `analyticalElement.m`, some constants are converted to vectors in lines 64-66. Finally, before starting the optimisation loop, some problem information is output to the command window in lines 67-71.

## 1.3 Optimisation loop (lines 72-160)

Before the optimisation loop begins, timers are started for timing each iteration and the full optimisation process:

```
73 destime = tic; ittime = tic;
```

The optimisation loop is started using a `while` command and plotting the design field if requested:

```
74 while (loop ≤ maxiter)
75     if (plotdes); figure(1); imagesc(xPhys); colorbar; ...
           caxis([0 1]); axis equal; axis off; drawnow; end
```

where `loop` is the design iteration counter.

The greyscale indicator introduced by ? is computed for the current design field:

```
76     %% GREYSCALE INDICATOR
77     Md = 100*full(4*sum(xPhys(:).*(1-xPhys(:)))/neltot);
```

Then the Brinkman penalisation factor and its design derivative is computed for all elements:

```
78     %% MATERIAL INTERPOLATION
79     alpha = alphamin + ...
           (alphamax-alphamin)*(1-xPhys(:))./(1+qa*xPhys(:));
80     dalpha = (qa*(alphamax - alphamin)*(xPhys(:) - ...
           1))./(xPhys(:)*qa + 1).^2 - (alphamax - ...
           alphamin)./(xPhys(:)*qa + 1);
```

### 1.3.1 Newton solver (lines 81-112)

The Newton solver is initiated for the current design iteration:

```
81     %% NON-LINEAR NEWTON SOLVER
82     normR = 1; nlit = 0; fail = -1; nltime = tic;
83     while (fail ≠ 1)
84         nlit = nlit+1; nlittot = nlittot+1;
```

where `nlit` is the Newton iteration counter, `normR` is the relative norm of the current residual, `nltime` is the timer for the Newton solver, and `fail` is a flag indicating whether the algorithm has failed from both the previous solution and a zero solution (fail = 1).

The residual is built for the current Newton iteration using the `sparse` triplet function using values from the supplied vectorised element residual function `RES`:

```
85         % BUILD RESIDUAL AND JACOBIAN
86         sR = RES(dxv,dyv,muv,rhov,alpha(:)',S(edofMat'));
87         R = sparse(iR,jR,sR(:)); R(fixedDofs) = 0;
```

where the residual is set to zero at the fixed DOFs, because the update to the fixed DOFs should be zero as they have been seeded with the correct values in line 55. The initial residual norm `r0` is computed, if it is the first Newton iteration, otherwise, the relative norm `normR` is computed:

```
88         if (nlit == 1); r0 = norm(R); end
89         r1 = norm(R); normR = r1/r0;
```

The convergence of the non-linear solver will be plotted if requested (`plotres = 1`) and if the relative residual norm is below the required tolerance `nltol`, the solver is stopped:

```
90         if (plotres); figure(6); ...
               semilogy(nlittot,normR,'x'); axis square; grid ...
               on; hold on; end
91         if (normR < nltol); break; end
```

Subsequently, the Jacobian is built in a similar fashion from the supplied vectorised element Jacobian function `JAC` and corrected for boundary conditions using the nullspace matrices:

```
92         sJ = JAC(dxv,dyv,muv,rhov,alpha(:)',S(edofMat'));
93         J = sparse(iJ,jJ,sJ(:)); J = (ND'*J*ND+EN);
```

This ensures that the update will be zero for the fixed DOFs. Finally, the Newton step `dS` is found using the backslash operator:

```
94         % CALCULATE NEWTON STEP
```

```
95          dS = -J\R;
```

In order to determine the damping factor, the 2-norm line search is performed as described in Section 4.2 of the manuscript:

```
96          % L2-NORM LINE SEARCH
97          Sp = S + 0.5*dS;
98          sR = RES(dxv,dyv,muv,rhov,alpha(:)',Sp(edofMat'));
99          R = sparse(iR,jR,sR(:)); R(fixedDofs) = 0; r2 = norm(R);
100         Sp = S + 1.0*dS;
101         sR = RES(dxv,dyv,muv,rhov,alpha(:)',Sp(edofMat'));
102         R = sparse(iR,jR,sR(:)); R(fixedDofs) = 0; r3 = norm(R);
103         % SOLUTION UPDATE WITH "OPTIMAL" DAMPING
104         lambda = max(0.01,min(1.0,(3*r1 + r3 - 4*r2)/(4*r1 + ...
                4*r3 - 8*r2)));
```

and the damped Newton step is taken to update the solution:

```
105         S = S + lambda*dS;
```

Upon completion, information about the solution process is output in lines 110-111.

If problems are observed during the optimisation with non-convergence, the **plotres** variable can be set to 1 and the convergence of the residual norm will be plotted in line 90. If the Newton algorithm does not converge, then the Reynolds number might be too high and unsteady flow has been triggered. It may also be that the problem is just extremely non-linear and may benefit from slowly ramping up the inlet velocity. If the Newton solver fails to converge within **nlmax** iterations, the free DOFs are set to zero and the Newton solver is restarted:

```
106         % IF FAIL, RETRY FROM ZERO SOLUTION
107         if (nlit == nlmax && fail < 0); nlit = 0; ...
                S(freedofs) = 0.0; normR=1; fail = fail+1; end
108         if (nlit == nlmax && fail < 1); fail = fail+1; end
```

If the solver fails again from the zero solution, an error is declared and the code stops:

```
112     if (fail == 1); error('ERROR: Solver did not converge ...
            after retry from zero!\n      Stopping ...
            optimisation.\n'); end
```

### 1.3.2 Objective functional and volume constraint (lines 113-117)

The objective functional is evaluated using the supplied function `PHI` and the relative change from the previous design iteration is computed:

```
113 %% OBJECTIVE EVALUATION
114 obj = sum( PHI(dxv,dyv,muv,alpha(:)',S(edofMat')) );
115 change = abs(objOld-obj)/objOld; objOld = obj;
```

PHI is a vectorised function that returns all of the element contributions to the dissipated energy functional. The used volume is then found as the mean of the current design field, which is valid because all elements have the same volume:

```
116 %% VOLUME CONSTRAINT
117 V = mean(xPhys(:));
```

The performance of the current design and other statuses are output to the command window in lines 118-123.

### 1.3.3 Convergence check (lines 124-130)

Firstly, it is checked whether the relative change, **change**, in the objective functional is below the required limit, **chlim**. If so, the **chcnt** counter is increased by 1 and if not, the **chcnt** counter is reset. During the final continuation step, the optimisation process is stopped, if the relative change has been below the stopping criteria for the specified **chnum** number of iterations or if the number of iterations for the current step reaches :

```
124 %% EVALUATE CURRENT ITERATE - CONTINUE UNLESS CONSIDERED ...
      CONVERGED
125 if (change < chlim); chcnt = chcnt + 1; else; chcnt = 0; end
126 if (qastep == qanum && ( (chcnt == chnum) || (loopcont ...
      == conit) ) ); break; end
```

Otherwise, the optimisation process continues to compute the next design update and a header is output to the command window in lines 127-130.

### 1.3.4 Sensitivity analysis (lines 131-144)

Firstly, the right-hand side for the adjoint problem (RHS) must be assembled. This is done using the supplied vectorised function **dPHIds** that computes all element contributions to $\frac{\partial \phi}{\partial \mathbf{s}}$:

```
131 %% ADJOINT SOLVER
132 sR = [dPHIds(dxv,dyv,muv,alpha(:)',S(edofMat')); ...
      zeros(4,neltot)];
133 RHS = sparse(iR,jR,sR(:)); RHS(fixedDofs) = 0;
```

Then the transposed Jacobian, $\frac{\partial \mathbf{r}}{\partial \mathbf{s}}^T$, is built using the supplied vectorised function JAC and the adjoint solution is found using the backslash operator and stored in the vector $L$:

```
134     sJ = JAC(dxv,dyv,muv,rhov,alpha(:)',S(edofMat'));
135     J = sparse(iJ,jJ,sJ(:)); J = (ND'*J*ND+EN);
136     L = J'\RHS;
```

In order to compute the final sensitivities for the objective functional, the design derivatives of the residual, $\frac{\partial \mathbf{r}}{\partial \gamma}$, and the objective functional, $\frac{\partial \phi}{\partial \gamma}$, are required. These are built using the supplied vectorised function `dRESdg` and `dPHIdg`:

```
137     %% COMPUTE SENSITIVITIES
138     % OBJECTIVE
139     sR = ...
            dRESdg(dxv,dyv,muv,rhov,alpha(:)',dalpha(:)',S(edofMat'));
140     dRdg = sparse(iR(:),jE(:),sR(:));
141     dphidg = ...
            dPHIdg(dxv,dyv,muv,alpha(:)',dalpha(:)',S(edofMat'));
```

The senstivities are then found using Equation **??**:

```
142     sens = reshape(dphidg - L'*dRdg,nely,nelx);
```

Finally, the sensitivities of the volume constraint are simply set to $\frac{1}{n_{el}}$, since the volume is computed as the mean of all elements:

```
143     % VOLUME CONSTRAINT
144     dV = ones(nely,nelx)/neltot;
```

### 1.3.5 Optimality criteria update (lines 145-154)

First, the current design is copied to the vector to be updated (`xnew`) and the upper (`xupp`) and lower (`xlow`) limits of the updated design variables are computed:

```
145     %% OPTIMALITY CRITERIA UPDATE OF DESIGN VARIABLES AND ...
            PHYSICAL DENSITIES
146     xnew = xPhys; xlow = xPhys(:)-mvlim; xupp = xPhys(:)+mvlim;
```

Then the constant factor $x_e {B_e}^{\eta}$ from the OC update in Equation **??** is computed where $B_e$ is given by Equation **??**:

```
147     ocfac = xPhys(:).*max(1e-10,(-sens(:)./dV(:))).^(1/3);
```

The lower and upper bounds for the Lagrange multiplier, `l1` and `l2`, are defined as 0 and according to Equation **??**:

```
148     l1 = 0; l2 = ( 1/(neltot*volfrac)*sum( ocfac ) )^3;
```

The bisection algorithm is then run until the accuracy of the Lagrange multiplier is sufficient:

```
149     while (l2-l1)/(l1+l2) > 1e-3
150         lmid = 0.5*(l2+l1);
151         xnew(:) = ...
                max(0,max(xlow,min(1,min(xupp,ocfac/(lmid^(1/3))))));
152         if mean(xnew(:)) > volfrac; l1 = lmid; else; l2 = ...
                lmid; end
153     end
```

where **xnew** is updated iteratively according to the rule in Equation ??. Finally, the updated design field is saved in **xPhys** on line 154.

### 1.3.6 Continuation scheme update (lines 155-159)

After finishing the design update for the current iteration for a given continuation step, if the maximum number of iterations has been reached or the change in objective function has been below the stopping criteria sufficiently, the next continuation step is taken:

```
155     %% CONTINUATION UPDATE
156     if (qastep < qanum && (loopcont == conit || chcnt == ...
            chnum) )
157         loopcont = 0; chcnt = 0;
158         qastep = qastep + 1; qa = qavec(qastep);
159     end
```

## 1.4 Post-processing (lines 161-170)

When the optimisation process is complete, the final information is output to the command window in lines 161-167. Subsequently, the optimised design and state fields are visualised in plots, which takes place in a separate MATLAB script **postproc.m** (detailed in Section 3) in order to keep the main code clean and concise:

```
168 %% PLOT RESULTS
169 run('postproc.m');
```

# 2 Detailed description of problems.m

The problem definition script contains two problems, where the setup of the double pipe problem will be covered here. First, the problem specified by the user in the variable **probtype** is chosen:

```
if (probtype == 1) % DOUBLE PIPE PROBLEM
```

Some checks are made of the defined mesh to ensure that the number of elements fits the specified boundary conditions and that sufficient number of elements are used:

```
    if ( mod(nely,6) > 0 > 0 )
        error('ERROR: Number of elements in y-dir. must be ...
            divisable by 6.');
    elseif ( nely < 30 )
        error('ERROR: Number of elements in y-dir. must be ...
            above 30.');
    end
```

Then, the size and position of the inlets and outlets are defined:

```
    inletLength = 1/6*nely; inlet1 = 1/6*nely+1; inlet2 = ...
        4/6*nely+1;
    outletLength = 1/6*nely; outlet1 = 1/6*nely+1; outlet2 = ...
        4/6*nely+1;
```

where `inletLength` and `outletLength` are the size of the inlets and outlets, respectively, `inlet1` and `inlet2` are the starting positions of the first and second inlet, respectively, and `outlet1` and `outlet2` are the starting positions of the first and second outlet, respectively. All dimensions are here given in terms of elements. The nodes belonging to the inlet, outlet, top and bottom, left and right boundaries, respectively, are then found as:

```
    nodesInlet   = [inlet1:(inlet1+inletLength)' ...
        inlet2:(inlet2+inletLength)'];
    nodesOutlet = ...
        (nodx-1)*nody+[outlet1:(outlet1+outletLength)' ...
        outlet2:(outlet2+outletLength)'];
    nodesTopBot = [1:nely+1:nodtot nody:nody:nodtot];
    nodesLefRig = [2:nely (nelx)*nody+2:nodtot-1];
```

The fixed DOFs are then calculated for each subsection:

```
    fixedDofsTBx = 2*nodesTopBot-1; fixedDofsTBy = ...
        2*nodesTopBot;
    fixedDofsLRx = 2*setdiff(nodesLefRig,[nodesInlet ...
        nodesOutlet])-1;
    fixedDofsLRy = 2*nodesLefRig;
    fixedDofsInX  = 2*nodesInlet-1; fixedDofsInY  = ...
        2*nodesInlet;
    fixedDofsOutY = 2*nodesOutlet; fixedDofsOutP = ...
        2*nodtot+nodesOutlet;
```

It should be noted that for the problem at hand, no-slip and no-penetration will be imposed on all boundaries, except for: the inlet, where a normal velocity will be imposed in the $x$-direction (`fixedDofsInX`) and a zero tan-

gential velocity will be imposed in the $y$-direction (`fixedDofsInY`); and the outlet, where a zero tangential velocity will be imposed in the $y$-direction (`fixedDofsOutY`) and a zero pressure will be imposed (`fixedDofsOutP`). Thereafter, these are collected:

```
    fixedDofsU = [fixedDofsTBx fixedDofsTBy fixedDofsLRx ...
       fixedDofsLRy ...
                 fixedDofsInX fixedDofsInY fixedDofsOutY];
    fixedDofsP = [fixedDofsOutP];
    fixedDofs  = [fixedDofsU fixedDofsP];
```

where `fixedDofsU`, `fixedDofsP` and `fixedDofs` contain all fixed DOFs for velocity, pressure and both, respectively.

A vector containing the corresponding values of the prescribed nodal velocity is then defined:

```
    % DIRICHLET VECTORS
    u = @(y) -4*y.^2+4*y; Uinlet = ...
       Uin*u([0:inletLength]'/inletLength);
    DIRU=zeros(nodtot*2,1); DIRU(fixedDofsInX) = [Uinlet' ...
       Uinlet'];
    DIRP=zeros(nodtot,1); DIR = [DIRU; DIRP];
```

where the prescribed inlet distribution is defined as a parabola evaluated at the nodal points of the inlets. The vectors `DIRU` and `DIRP` contains all zeroes, except for DOFs where a Dirichlet values is to be prescribed. The vector `DIR` is the collection of these two vectors for the whole system. The Reynolds number for the problem is computed, here based on the inlet flow and inlet dimension:

```
    % INLET REYNOLDS NUMBER
    Renum = Uin*(inletLength*Ly/nely)*rho/mu;
```

Finally, additional problems can then be implemented by adding `elseif` statements:

```
elseif (probtype == 2) % PIPE BEND PROBLEM
```

# 3 Detailed description of `postproc.m`

In the post-processing file, the design field, the Brinkman penalty factor (in logarithmic scale), the velocity magnitude field and the pressure field are plotted for the final design:

```
%% POST-PROCESSING
% SETTING UP NODAL COORDINATES FOR STREAMLINES
```

```
[X,Y] = meshgrid(0.5:nodx,0.5:nody); sx = 0.5*ones(1,21); sy ...
    = linspace(0,nody,21);
U = S(1:(nely+1)*(nelx+1)*2); ...
    umag=reshape(sqrt(U(1:2:end).^2+U(2:2:end).^2),nely+1,nelx+1);
% DESIGN FIELD
figure(1); imagesc(xPhys); colorbar; caxis([0 1]); axis ...
    equal; axis off;
h = ...
    streamline(X,Y,reshape(U(1:2:end),nody,nodx),-reshape(U(2:2:end),nody,nodx),sx,
    set(h,'Color','black');
% BRINKMAN PENALTY FACTOR
figure(2); imagesc(reshape(log10(alpha),nely,nelx)); ...
    colorbar; caxis([0 log10(alphamax)]); axis equal; axis ...
    off; %colormap turbo;
% VELOCITY MAGNITUDE FIELD
figure(3); imagesc(umag); colorbar; axis equal; axis on; ...
    hold on; %colormap turbo;
h = ...
    streamline(X,Y,reshape(U(1:2:end),nody,nodx),-reshape(U(2:2:end),nody,nodx),sx,
    set(h,'Color','black');
% PRESSURE FIELD
P = S(2*nodtot+1:3*nodtot);
figure(4); imagesc(reshape(P,nody,nodx)); colorbar; axis ...
    equal; axis off; %colormap turbo;
h = ...
    streamline(X,Y,reshape(U(1:2:end),nody,nodx),-reshape(U(2:2:end),nody,nodx),sx,
    set(h,'Color','black');
```

Lastly, the velocity and design field across a line through the domain is plotted:

```
% VELOCITY ALONG A LINE
if (probtype == 2)
    uline=flipud(diag(fliplr(umag))); ...
        xline=flipud(diag(fliplr(xPhys)));
else
    uline=umag(:,floor((end-1)/2)); xline=xPhys(:,floor(end/2));
end
figure(5);
subplot(3,1,1); plot(uline,'-x'); grid on;
subplot(3,1,2); plot(log10(uline),'-x'); grid on;
subplot(3,1,3); plot(xline,'-x'); grid on; drawnow
```

where a vertical line halfway along the $x$-axis is plotted for the first problem and the diagonal is plotted for the second problem.

Finally, if `exportdxf = 1`, the design contour will be exported as an DXF file in the separate MATLAB script `export.m`:

```
if (exportdxf); run('export.m'); end
```

This script is not covered herein, since it is not important for the topology optimisation. It seems to work most of the time for open internal channel designs, but does not provide a closed loop for freely floating objects in external flow.

# 4 Detailed description of `analyticalElement.m`

This script uses the MATLAB Symbolic Toolbox to derive the finite element vectors and matrices, as well as the necessary partial derivatives using symbolic differentiation.

At the top of the document, a few flags select what should be done:

```
%% Switches
buildJR = 1; exportJR = 1;
buildPhi = 1; exportPhi = 1;
```

where `buildJR` and `exportJR` determine whether the residual and Jacobian should be built and exported, respectively, and `buildPhi` `exportPhi` determine whether the functional and its derivatives should be built or exported, respectively. Building and exporting the residual and Jacobian can takes a very long time due the complicated finite element formulation. So if you are changing the objective functional, it is a good idea to turn off the building and exporting of the residual and Jacobian after the first time.

The algebraic variables used need to be initialised as symbolic variables:

```
%% Initialisation
syms rho mu alpha dalpha xi eta dx dy;
syms u1 u2 u3 u4 u5 u6 u7 u8 p1 p2 p3 p4;
```

## 4.1 Residual and Jacobian

The shape functions and defined as bi-linear and the shape function matrices for the velocity, `Nu`, and pressure, `Np`, are built:

```
%% Shape functions and matrices
xv = [-1 1 1 -1]'; yv = [-1 -1 1 1]';
Np = 1/4*(1+xi*xv').*(1+eta*yv');
Nu = sym(zeros(2,8));
Nu(1,1:2:end-1) = Np;
Nu(2,2:2:end) = Np;
```

The elements are defined as rectangular ones `dx` wide and `dy` tall and the origin is placed in the centre. The nodal co-ordinates are defined and the element isoparametric Jacobian is computed:

```
%% Nodal coordinates, interpolation and coordinate transforms
xc = dx/2*xv; yc = dy/2*yv;
x = Np*xc; y = Np*yc;
J = [diff(x,xi) diff(y,xi); diff(x,eta) diff(y,eta)];
iJ = inv(J); detJ = det(J);
```

In principle the current script can be generalised to arbitrary quadrilateral elements.

The derivatives of the shape functions are pre-computed and stored:

```
%% Derivatives of shape functions
dNpdx = iJ(:,1)*diff(Np,xi) + iJ(:,2)*diff(Np,eta);
dNudx = sym(zeros(2,8,2));
for i = 1:2
   dNudx(i,:,:) = transpose(iJ(:,1)*diff(Nu(i,:),xi) + ...
       iJ(:,2)*diff(Nu(i,:),eta));
end
```

The vectors of nodal DOFs are defined and the derivatives of the velocity, **dudx**, and pressure, **dpdx**, are computed:

```
%% Nodal DOFs
u = [u1; u2; u3; u4; u5; u6; u7; u8];
p = [p1; p2; p3; p4]; s = [u; p];
ux = Nu*u; px = Np*p;
dudx = [dNudx(:,:,1)*u dNudx(:,:,2)*u];
dpdx = dNpdx*p;
```

The stabilisation parameters are calculated according to Appendix B of the manuscript:

```
%% Stabilisation parameters
h = sqrt(dx^2 + dy^2);
u0 = subs(ux,[xi,eta],[0,0]);
ue = sqrt(transpose(u0)*u0);
tau1 = h/(2*ue);
tau3 = rho*h^2/(12*mu);
tau4 = rho/alpha;
tau  = (tau1^(-2) + tau3^(-2) + tau4^(-2))^(-1/2);
```

The residual vectors are built by looping through all the indices of the weak form equations in Appendix B of the manuscript:

```
    Ru = sym(zeros(8,1)); Rp = sym(zeros(4,1));
    % Momentum equations
    for g = 1:8
        for i = 1:2
            Ru(g) = Ru(g) + alpha*Nu(i,g)*ux(i); % Brinkman term
            for j = 1:2
```

```
                Ru(g) = Ru(g) + mu*dNudx(i,g,j)*( dudx(i,j) ...
                    + dudx(j,i) ); % Viscous term
                Ru(g) = Ru(g) + rho*Nu(i,g)*ux(j)*dudx(i,j); ...
                    % Convection term
                Ru(g) = Ru(g) + ...
                    tau*ux(j)*dNudx(i,g,j)*alpha*ux(i); % ...
                    SUPG Brinkman term
                for k = 1:2
                    Ru(g) = Ru(g) + ...
                        tau*ux(j)*dNudx(i,g,j)*rho*ux(k)*dudx(i,k); ...
                        % SUPG convection term
                end
                Ru(g) = Ru(g) + ...
                    tau*ux(j)*dNudx(i,g,j)*dpdx(i); % SUPG ...
                    pressure term
            end
            Ru(g) = Ru(g) - dNudx(i,g,i)*px; % Pressure term
        end
    end
    % Incompressibility equations
    for g = 1:4
        for i = 1:2
            Rp(g) = Rp(g) + Np(1,g)*dudx(i,i); % Divergence term
            Rp(g) = Rp(g) + tau/rho*dNpdx(i,g)*alpha*ux(i); ...
                % PSPG Brinkman term
            for j = 1:2
                Rp(g) = Rp(g) + ...
                    tau*dNpdx(i,g)*ux(j)*dudx(i,j); % PSPG ...
                    convection term
            end
            Rp(g) = Rp(g) + tau/rho*dNpdx(i,g)*dpdx(i); % ...
                PSPG pressure term
        end
    end
```

The algebraic expressions from the above nested loops will be very long and complicated. Thus, a simplification is necessary:

```
    fprintf('Simplifying Ru... \n');
    Ru = simplify(detJ*Ru);
    fprintf('Simplifying Rp... \n');
    Rp = simplify(detJ*Rp);
```

This simplification will significantly reduce the number of code lines of the exported functions. Beware that this step can take a long time due to the complexity of the finite element formulation.

Since the elements are defined to be rectangular, the residual can be analytically integrated:

```
    %% Integrate analytically
    fprintf('Integrating Ru... \n');
    Ru = int(int(Ru,xi,[-1 1]),eta,[-1 1]);
    fprintf('Integrating Rp... \n');
    Rp = int(int(Rp,xi,[-1 1]),eta,[-1 1]);
    fprintf('Simplifying Ru... \n');
    Ru = simplify(Ru);
    fprintf('Simplifying Rp... \n');
    Rp = simplify(Rp);
```

Beware that this step can also take a long time due to the complexity of the finite element formulation.

To form the Jacobian for the Newton solver and the adjoint problem, the residual is symbolically differentiated automatically:

```
    %% Differentiate residual to form Jacobian
    Re = [Ru; Rp];
    Je = sym(zeros(12,12));
    for b = 1:12
        fprintf('Computing dR/ds%2i... \n',b);
        Je(:,b) = diff(Re,s(b));
    end
```

Beware that this step can also take a long time due to the complexity of the finite element formulation.

The last step is to export the residual and Jacobian to vectorised MATLAB functions:

```
%% Export residual and Jacobian
if (exportJR)
    fprintf('Exporting residual... \n');
    f = matlabFunction(Re,'File','RES','Comments','Version: ...
        0.99','Vars',{dx,dy,mu,rho,alpha,transpose([u1 u2 u3 ...
        u4 u5 u6 u7 u8 p1 p2 p3 p4])});
    fprintf('Exporting Jacobian... \n');
    f = ...
        matlabFunction(Je(:),'File','JAC','Comments','Version: ...
        0.99','Vars',{dx,dy,mu,rho,alpha,transpose([u1 u2 u3 ...
        u4 u5 u6 u7 u8 p1 p2 p3 p4])});
end
```

Beware that this step can also take a long time due to the complexity of the finite element formulation.

## 4.2 Optimisation related quantities

The objective functional is defined as the loop over the indices of the definition in Equation 20 (Section 5.1) of the manuscript:

```
    %% Compute objective functional
    fprintf('Computing phi... \n');
    phi = 1/2*alpha*transpose(ux)*ux;
    for i = 1:2
        for j = 1:2
            phi = phi + 1/2*mu*dudx(i,j)*( dudx(i,j) + ...
                dudx(j,i) );
        end
    end
```

and subsequently analytically integrated and simplified:

```
    %% Intregrate and simplify objective functional
    fprintf('Integrating phi... \n');
    phi = int(int(detJ*phi,xi,[-1 1]),eta,[-1 1]);
    phi = simplify(phi);
```

The partial derivates of the functional with respect to the design and state fields are then computed automatically using symbolic differentiation:

```
    %% Compute the partial derivative wrt. design field
    fprintf('Computing dphi/dgamma... \n');
    dphidg = simplify( diff(phi,alpha)*dalpha );
    %% Compute the partial derivative wrt. state field
    dphids = sym(zeros(12,1));
    for a = 1:12
        fprintf('Computing dphi/ds%2i... \n',a);
        dphids(a) = simplify(diff(phi,s(a)));
    end
```

For adjoint sensitivity analysis, we also need the partial derivative of the residual vector with respect to the design field:

```
%% Compute partial derivative of residual wrt. design field
if (buildJR)
    fprintf('Computing dr/dgamma... \n');
    drdg = simplify( diff(Re,alpha)*dalpha );
end
```

Finally, these required quantities and vectors are exported to vectorised MATLAB functions:

```
%% Export optimisation functions
if (exportPhi)
    fprintf('Exporting phi... \n');
    f = matlabFunction(phi,'File','PHI','Comments','Version: ...
        0.9','Vars',{dx,dy,mu,alpha,transpose([u1 u2 u3 u4 u5 ...
        u6 u7 u8 p1 p2 p3 p4])});
    fprintf('Exporting dphi/dg... \n');
    f = ...
        matlabFunction(dphidg,'File','dPHIdg','Comments','Version: ...
```

```
        0.9','Vars',{dx,dy,mu,alpha,dalpha,transpose([u1 u2 ...
        u3 u4 u5 u6 u7 u8 p1 p2 p3 p4])});
    fprintf('Exporting dphi/ds... \n');
    f = ...
        matlabFunction(dphids(1:8),'File','dPHIds','Comments','Version: ...
        0.9','Vars',{dx,dy,mu,alpha,transpose([u1 u2 u3 u4 u5 ...
        u6 u7 u8 p1 p2 p3 p4])});
end
if (exportJR)
    fprintf('Exporting dr/ds... \n');
    f = ...
        matlabFunction(drdg,'File','dRESdg','Comments','Version: ...
        0.9','Vars',{dx,dy,mu,rho,alpha,dalpha,transpose([u1 ...
        u2 u3 u4 u5 u6 u7 u8 p1 p2 p3 p4])});
end
```
